# Supplementary material for: Post-Quantum VRF and its Applications in Future-Proof Blockchain System
Source: arXiv:2109.02012 source file (2021-09-05)
Supplement: Supplementary file 1 [file Appendix-comitment.tex]

% !TEX encoding =UTF-8 Unicode
%!TEX root = ../mainVRFarxiv.tex

\subsection{One-Time Signature}
One-time signature (OTS) schemes are digital signature constructions in themselves, but any OTS signature reveals part of the associated secret key. Consequently, every OTS secret key can only be used once. Indeed, a second signature using the same
key would reveal even more about the key, allowing further signatures to be forged. Two well-known OTS schemes are the Lamport-Diffie scheme~\cite{Lamport79} and the Winternitz scheme~\cite{IMA:DodSmaSta05}. Their structure is similar, and their security requirement reduces the collision resistance of the used hash function. In both cases,
\begin{itemize}
  \item signing keys are randomly generated, and
  \item the corresponding verification key is obtained by applying a one-way function (repeatedly, in the Winternitz case) to the signing key.
\end{itemize}
As it is usual for signature schemes, in both cases, signatures on a message are actually applied to the hash of the message.

\noindent\textbf{Lamport Signature Scheme}
In Lamport's scheme, the public key consists of two hash outputs for secret inputs; to sign a bit $0$, reveal the pre-image of the first output; to sign a bit $1$, reveal the pre-image of the second output. Obviously, the secret key in this scheme can be used only once: signing a total of $T$ bits of messages requires a sequence of $T$ public keys and is therefore highly impractical.

\mybox{Lamport Signature Scheme.}{white!40}{white!10}{
One-time signature (OTS) scheme was proposed by Lamport in 1979. Meanwhile, use cryptographic hash function h with 256-bit output.
\small
%\scriptsize
%\smallskip
\vspace{-8pt}
\begin{itemize}
\item \textbf{Key Generation.} $\Gen(1^{\secp})$.
\begin{enumerate}
  \item Choose private key: (pseudo-)random
\begin{equation*}
  \bigparens{(\sksub{0,0}, \sksub{0,1}), (\sksub{1,0}, \sksub{1,1}), (\sksub{2,0}, \sksub{2,1}),\cdots, (\sksub{255,0}, \sksub{255,1})}
\end{equation*}
where each $\sksub{i,j}\in \set{0, 2^{256}-1}$.
  \item Generate the public key
  \begin{equation*}
  \Bigparens{\bigparens{\hashH(\sksub{0,0}), \hashH(\sksub{0,1})}, \bigparens{\hashH(\sksub{1,0}), \hashH(\sksub{1,1})}, \bigparens{\hashH(\sksub{2,0}), \hashH(\sksub{2,1})},\cdots, \bigparens{\hashH(\sksub{255,0}),\hashH(\sksub{255,1})}}.
\end{equation*}
\end{enumerate}

\item \textbf{Signing.} $\Sign(\cdot)$.
\begin{itemize}
  \item Sign messages (hashes) of 256 bits $(\msg_0,\cdots, \msg_{255})$.
  \item Then, for each bit in the hash, based on the value of the bit, the algorithm picks one number from the corresponding pairs of numbers that make up its private key (\ie, if the bit is 0, the first number is chosen, and if the bit is 1, the second is chosen). This produces a sequence of 256 random numbers. Thus, signature is $(\signsub{0,m_0}, \signsub{1,m_1}, \signsub{2, m_2}, \cdots,  \signsub{255, m_{255}})$.
\end{itemize}
As each number is itself 256 bits long, the total size of the signature will be 256×256 bits = 8 KB.

\item \textbf{Verification.} $\Vrfy(\cdot)$. Compare hashes of signature components to elements of the public key.

\end{itemize}
\noindent{\textbf{Remark.}}
Secure only for a signature on one message and 16KB private and public key, 8 KB signature.
}{Lamport Signature Scheme.~\label{fig:Lamport-signature.}}

\subsubsection{Winternitz one-time signature scheme}

Before describing our scheme, we first use the notation $f^i_k(x)$ to denote that the function is iterated $i$ times on input $x$ using key $k$ for the first iteration and the output of the function as a key for the next iteration,
\begin{equation*}
  f^2_{k}(x)=f_{f_k(x)}(x)=f(f_k(x)) \text{~and~} f^0_k(x)=x.
\end{equation*}

In the following, we only describe the generation of signatures for $m$-bit messages. The generalization to arbitrary sized messages is straight forward by utilizing a collision resistant hash function.

\mybox{Winternitz one-time signature scheme.}{white!40}{white!10}{
\small
%\scriptsize
%\smallskip
\vspace{-8pt}
\begin{itemize}
\item \textbf{Key Generation.} $\Gen(1^{\secp})$.

\begin{enumerate}
  \item First we choose the Winternitz parameter $w \in N, w > 1$, defining the compression level.
  \item Next we choose a random value $x\gets\set{0,1}^n$. The signature key consists of $\ell$ bit strings of length $n$ chosen uniformly with the random distribution,
      \begin{equation*}
        \sk=(\sk_1,\sk_2,\cdots,\sk_{\ell})\in\set{0,1}^{(n,\ell)}
      \end{equation*}
      where $\ell=\ell_1+\ell_2$ is computed as follows.

 \item The verification key is computed using functions from the family $\calF(n)$. The bit strings in the signature key are used as a key for the function $\hashF$ and the function is iterated $w-1$ times on input $x$.
      \begin{equation*}
        \pk=(\pk_0,\pk_1,\cdots, \pk_{\ell})=(x,\hashFsub{\sk_1}(x), \hashFsub{\sk_2}(x),\cdots, \hashFsub{\sk_{\ell}}(x) )
      \end{equation*}
 \end{enumerate}

\item Signature generation $\Sign(\cdot)$.
\begin{enumerate}
  \item We describe how to sign an $m$-bit message $\msgM = (\msgM_1,\cdots, \msgM_{\ell_1})$ given in base-$w$ representation, \ie,
       $\msgM_i \in\set{0,\cdots,w-1}$ for $i = 1, \cdots, \ell_1$. We begin by computing the checksum
       \begin{equation*}
         \checksum=\sum_{i=1}^{\ell_1}(w-1-\msgM)
       \end{equation*}
       and represent it to base $w$ as $\checksum=(\checksum_1, \checksum_2, \cdots, \checksum_{\ell_2})$.
       The length of the base-$w$ representation of $\checksum$ is at most $\ell_2$ since $\checksum \leq \ell(w-1)$. Then we set $B=(b_1,\cdots, b_{\ell})=\msgM \|\checksum$. The signature of message $\msgM$ is computed as
       \begin{equation*}
         \sign:=(\signsub{1}, \signsub{2}, \cdots, \signsub{\ell})=(\hashFsupb{b_1}{\sk_1}(x), \hashFsupb{b_2}{\sk_2}(x),\cdots, \hashFsupb{b_{\ell}}{\sk_{\ell}}(x) )
       \end{equation*}

  \item Signature verification (Algorithm $\Vrfy$.)
      \begin{enumerate}
     \item    The verifier first computes the base-$w$ string $B=(b_1,\cdots,b_{\ell})$ as described above. Then he checks whether
         \begin{equation*}
           \bigparens{\hashFsupb{w-1-b_1}{\sigma_1}(\pk_0),\hashFsupb{w-1-b_2}{\sigma_2}(\pk_0),\cdots, \hashFsupb{w-1-b_{\ell}}{\sigma_{\ell}}(\pk_0)}\overset{?}{=} (\pk_1,\pk_2,\cdots, \pk_{\ell}).
         \end{equation*}
        The signature is accepted iff the comparison holds.
   \end{enumerate}

\end{enumerate}

\end{itemize}
}{Winternitz one-time signature scheme.~\label{fig:Winternitz-signature.}}

\subsection{Merkle Tree}

Merkle trees~\cite{C:Merkle89} are also called \emph{hash trees} because nodes are computed through hashing and concatenation. The leaves of the tree are the hashed OTS verification keys (\ie, OTS public keys). Signatures contain both an OTS signature and a way to authenticate this OTS signature against the public key of the entire tree.

HBS schemes can provide a valuable property: forward security~\cite{XXX} that all signatures generated before a key compromise remain valid. This attribute supports a form of long-term security.

\zlinote{
 Note that forward security is not an intrinsic property of HBS; it requires special constructs such as the use of a pseudo-random number generator. Since these constructs also provide other advantages (such as reduced storage requirements), there is much incentive to use them.
}

As a consequence, HBS schemes are said to be \emph{stateful}. Statefulness is inconvenient in practice for a number of reasons.
\begin{itemize}
  \item First, it does not fit common software interfaces.
  \item Second, performance is impacted by frequent key access.
  \item Besides, key storage conditions become critical. Copies or backups containing keys, and old key states in general, must be avoided for security reasons.
\end{itemize}
These concrete consequences need to be taken into account when developing mitigation strategies. \emph{Stateless} HBS (namely that SPHINCS), based on random index selection and a few-time signature scheme, has recently been introduced~\cite{EC:BHHLNP15} to circumvent this issue.

\subsection{Recap: Sigmal-protocol, Unrush's Transform and Play-MPC-in-the-head}

\subsubsection{Sigma Protocol}

\mybox{Sigma Protocol.}{white!40}{white!10}{
\small
%\scriptsize
%\smallskip
\vspace{-1.6pt}
A sigma protocol (or $\Sigma$-protocol) is a three flow protocol between a prover $\Prove$ and a verifier $\Verify$, where transcripts have the form $(\mask, \chlg, \resp)$. Let $f$ be a relation such that $f(\wits)=\stmt$, where $y$ is common input and $\wits$ is a witness known only to $\Prove$. $\Verify$ accepts if $\phi(y, \mask, \chlg, \resp)=1$ for an efficiently computable predicate $\phi$.
\begin{itemize}
\item prover samples a mask (\ie, a random number) $\mask$ to disguise the witness $\wits$ and computes $a=f(\mask)$, then sends $a$ to the verifier.
\item upon receiving $a$ from the prover, the verifier chooses a challenge $\chlg$ from the challenge space.
\item prover generates the response $\resp:=\chlg\cdot \wits + \mask$.
\item verifier checks $f(\resp)=\chlg\cdot \stmt+a$.
\end{itemize}
Further, there exists an efficient simulator, given $\stmt$ and a randomly chosen
}{Sigma Protocol.~\label{fig:Fish-signature.}}

\subsubsection{Unrush's Transform.}

\mybox{Unrush's Transform.}{white!40}{white!10}{
\small
%\scriptsize
%\smallskip
\vspace{-1.6pt}
Given a $\Sigma$-protocol with challenge space $\chlgspace$, an integer $t$, a statement $\stmt$, and a random permutation $\perm$, the prover will
\begin{itemize}
\item Run the first phase of the $\Sigma$-protocol $t$ times to produce $\rand_1, \rand_2, \cdots, \rand_t$.
\item For each $i\in\set{1, 2, \cdots, t}$, and for each $j\in \chlgspace$, compute the response $\resp_{i,j}$ for $\rand_i$ and challenge $j$. Compute $g_{i,g}=\perm(\resp_{i,j})$.
\item Compute $\hashH(\stmt, \rand_1, \rand_2, \cdots, \rand_t, g_{1,1}), g_{1,2}, g_{t\abs{\chlgspace}}$ to obtain a set of indices $J_1, J_2, \cdots, J_t$.
\item output proof $\zkproof$

\end{itemize}

}{Unrush's Transform.~\label{fig:Fish-signature.}}

\mybox{Picnic: Honest-verifier Zero-knowledge.}{white!40}{white!10}{
\small
%\scriptsize
%\smallskip
\vspace{-8pt}
\begin{itemize}
\item $\Gen(1^{\secp})$. Choose a secret key $s$

\item $\Sign()$.
\item $\Vrfy()$.
\end{itemize}

}{Picnic: Honest-verifier Zero-knowledge.~\label{fig:Fish-signature.}}

\subsubsection{ZKBoo atop IKOS}
The famous IKOS (\ie, Ishai, Kushilevitz, Ostrovsky, Sahai)~\cite{STOC:IOHK07} proposed in STOC2007 a method (play-MPC-in-the-head) to obtain zero-knowledge from MPC. Plugging the right MPC protocol, we can get a nearly practical zero-knowledge protocol with very good asymptotic complexity (\ie, proving time much smaller than SNARG).

$\ZKBoo$~\cite{USEUSENIX:GiaMadOrl16} means \textit{zero-knowledge for Boolean circuits} which can be seen as a generalization, simplification, and implementation of IKOS with the sole goal of practical efficiency.
In IKOS, we assume that the statement $\stmt\in\calL$ is the public input of the ZK protocol, while the witness $\wits$ is the private input of the prover (\ie, $R(\stmt, \wits)=1$).

\begin{definition}[$\prod_{f}$]
Let $\prod_{f}$ be an MPC protocol that realizes any $n$-party function $f$ with perfect correctness.
\end{definition}

\begin{itemize}
  \item A prover simulates an MPC protocol between a number of ``virtual'' servers (at least 3) and then commits to the views and the internal state of the individual servers.
  \item The verifier challenges the prover by asking to open a subset of these commitments.
\end{itemize}

\mybox{IKOS Protocol.}{white!40}{white!10}{
\small
%\scriptsize
%\smallskip

The verifier and the prover have input $\stmt\in \calL$. The prover knows $\wits$ such that $R(\stmt, \wits)=1$. A perfectly correct and $t$-private $n$-party MPC protocol $\prod_{f_\stmt}$ is given ($2 \leq t < n$).

\vspace{-5pt}
\begin{itemize}
\item \textbf{Commit}.  The prover does the following:
\begin{enumerate}
  \item  Sample random numbers $\wits_1,\wits_2,\cdots,\wits_n$ \suchthat~ $\wits_1\oplus\wits_2\oplus\cdots\oplus \wits_n=\wits$;
  \item Consider the $n$-input function $f_{\stmt}$ defined as
  \[
  f_{\stmt}(\wits_1,\cdots,\wits_n)
      :=R(\stmt,\wits_1\oplus\wits_2\oplus\cdots\oplus \wits_n)
  \]
  and emulates ``in his head'' $\prod_{f_\stmt}(\wits_1,\wits_2,\cdots,\wits_n)$. After the emulation, the prover obtains the views $c_i=\view_{\Prove_i}(\wits)$ for all $i\in [n]$;
  \item Compute the commitments to each of the $n$ produced views $c_1, c_2, \cdots, c_n$ \ie, $\Com(c_1), \Com(c_2), \cdots, \Com(c_n)$.
\end{enumerate}

\item \textbf{Challenge}. After all the commitments have been stored, the verifier challenges the prover to open some of these commitments. The verifier chooses a subset $E\subseteq [n]$ such that $\abs{E}=t$ and sends it to the prover.

\item \textbf{Prove}. The prover opens the requested commitments and reveals the value $c_e$ for all $e\in E$.
\item \textbf{Verify}. The verifier runs the following checks:
\begin{enumerate}
  \item If $\exists~e\in E$ \suchthat~ $\prod_{f_\stmt}(\view_{\Prove_e}(\wits))\neq 1$, output $\Reject$.
  \item If $\exists~\set{i,j}\subset E$ \suchthat $\view_{\Prove_i}(\wits)$ is not consistent with $\view_{\Prove_j}(\wits)$, output $\Reject$.
  \item Output $\Accept$. Namely that, if and only if all the opened views are consistent with each other and with output 1.
\end{enumerate}
\end{itemize}
}{The IKOS zero-knowledge protocol for the relation $R$ in the commitment-hybrid model.~\label{fig:Fish-signature.}}

\begin{figure}[ht]
  \centering
  \includegraphics[width=0.6\textwidth]{{ZKBoo.png}}
  \vspace{-10pt}
  \caption{ZKBoo via Play-MPC-in-the-head}\label{fig:ZKBoo}
\end{figure}

\subsubsection{\ZKBpp atop IOKS and ZKBoo}

$\ZKBpp$ is an improved version of ZKBoo with NIZK proofs that is less than half the size of ZKBoo proofs. Moreover, our benchmarks show that this size reduction comes at no extra computational cost.

\begin{itemize}
  \item \textbf{Privacy.}  The privacy guarantee of the underlying MPC protocol ensures that observing the state of a (sufficiently small) subset of servers does not reveal any information.
  \item \textbf{Correctness.} The correctness of the MPC protocol guarantees that if the prover tries to prove a false statement, then the joint views of some of the server must necessarily be inconsistent, and the verifier can check that efficiently.
\end{itemize}

The multiparty computation protocol (MPC) will implement the relation, and the input is the witness. For example, the MPC could compute $y = \SHA(x)$ where players each have a share of $x$ and $y$ is public.

The idea is to have the prover simulate a multiparty computation protocol ``in their head'', commit to the state and transcripts of all players, then have the verifier ``corrupt'' a random subset of the simulated players by seeing their complete state.

The verifier then checks that the computation was done correctly from the perspective of the corrupted players, and if so, he has some assurance that the output is correct and the prover knows $x$. Iterating this for many rounds then gives the verifier high assurance.

\subsection{Signature for Consensus}

``\emph{Picnic}''~(\ie,~\href{https://www.microsoft.com/en-us/research/project/picnic/}{https://www.microsoft.com/en-us/research/project/picnic/}) is the code name for a post-quantum digital signature algorithm, which is published at ACM CCS 2017. Picnic is developed in collaboration with researchers and engineers from Aarhus University, AIT Austrian Institute of Technology GmbH, Graz University of Technology, Microsoft Research, Princeton University, and the Technical University of Denmark.

\subsection{Zero-knowledge and its applications}
In this section, we review several of the building blocks used in our framework.

SNARKS (generic)

\begin{itemize}
  \item short proofs, efficient verification
  \item slow prover
  \item implementations: Pinocchio, libsnark
\end{itemize}

\noindent\textbf{Two protocols and one application}
Two protocols
\begin{itemize}
  \item ZKGC (from Garbled Circuits)
  \item ZKBoo (from MPC)
\end{itemize}

One application
\begin{itemize}
  \item Generic (post-quantum) signatures
\end{itemize}
