# Supplementary material for: Post-Quantum VRF and its Applications in Future-Proof Blockchain System
Source: arXiv:2109.02012 source file (2021-09-05)
Supplement: Supplementary file 2 [file Appendix-security.tex]

% !TEX encoding =UTF-8 Unicode
%!TEX root = ../mainVRFarxiv.tex
In this appendix, we detail the security for Subsection~\ref{subsec:secruityanalysis}. Before that, we first review some related notations in the following analysis.

\subsection{PoS Blockchain Syntax}

\begin{definition}[Adversaries Stake Ratio]
For any PPT adversary $\Adv$, the adversarial stake ratio $\strstkratio(\blockB):=\astkratio$, \wrt, blockchain $\blockB$ is defined as the ratio of $\Adv$'s total stake over the combined stake of all parties, as shown the following equality,
\begin{eqnarray*}
% \nonumber to remove numbering (before each equation)
  \strstkratio(\blockB) &=& \astkratio \\
  &=& \dfrac{\sum adversary's~ stakes}{\sum total~ stakerholder's~ stakes}\\
  &=& \dfrac{\sum_{j\in \bbS_{\Adv} }\stake_j}{\sum_{k=1}^n \stake_k}.
\end{eqnarray*}

%\begin{equation*}
%  \strstkratio(\blockB):=\astkratio = \dfrac{\sum                                   adversary's~ stakes}{\sum total~ stakerholder's~ stakes}= \dfrac{\sum_{j\in \bbS_{\Adv} }\stake_j}{\sum_{k=1}^n \stake_k}.
%\end{equation*}
\end{definition}

\begin{definition}[Leader Selection with Probability $\probld$] %~\cite[Ouroboros]{XXXX}

A leader $E_i$  with the pair verification key and stake $(\pk_i, \stake_i)$ is elected from the community of electors $\set{E_1, E_2, \cdots, E_n}$ with the probability
\begin{equation*}
  \probld_i =\dfrac{\stake_i}{\sum_{k=1}^n \stake_k},
\end{equation*}
where $\stake_i$ is the stake held by stakeholder $U_i$ (this is called ``weighting by stake'').
\end{definition}

\begin{theorem}[Chernof-Hoeffding Bound]\label{theorem:CHbound}
We define at least one honest party expects to gain the number of blocks at one round
  $p_i=\Ep[X_i]$.
Let $X_1, X_2, \cdots, X_T$ be independent random variables with $\Ep[X_i]$. Let $X=\sum^T_{i=1}X_i$ and $\mu=\sum^T_{i=1}p_i=\Ep[X]$. Then for all $\delta\geq 0$, we have that
\begin{equation*}
  \Pr[X\geq (1+\delta)\mu] \leq e^{-\frac{\delta^2}{2+\delta}\mu}
\end{equation*}
\text{~and~}
\begin{equation*}
\Pr[X\leq (1-\delta)\mu)] \leq e^{-\frac{\delta^2}{2+\delta}\mu}.
\end{equation*}
\end{theorem}
%
%\noindent\textbf{Epochs and Slots}. We adopt the same definition for transaction ledger properties as~\cite{C:KRDO17}. Eventually, the Ouroboros protocol divides the \textit{physical time} into \textit{epochs}, and each epoch is divided into \textit{slots}, and a slot is a relatively short period of time (for example, 20 seconds). Meanwhile, each slot has one and only one leader (slot leader, SL). The slot leader has a (sole) right to produce one and only one block during his slot. It means that the number of slot leaders is strictly equal to the number of slots in epoch (let's call this number $N$), so it is impossible to produce more than $N$ blocks during an epoch. If slot leader missed their slot (for example, when offline), the right to produce a block is lost until they are elected again. Notably, one or more slots can remain empty (without generated blocks), but the majority of blocks (at least $50\% + 1$) must be generated during an epoch.
%
%
%

%%
%%

\draft{
A protocol $\Pi$ implements a robust transaction ledger provided that the ledger that $\Pi$ maintains is divided into ``blocks'' (assigned to time slots) that determine the order with which transactions are incorporated in the ledger. It should also satisfy the following two properties.

\begin{itemize}
  \item \textbf{Persistence}. (Past (or stable) transactions in the ledger are immutable). Once a node of the system proclaims a certain transaction $\tx$ as \textit{stable}, the remaining nodes, if queried, will either report $\tx$ in the same position in the ledger or will not report as stable any transaction in conflict to $\tx$. Here the notion of stability is a predicate that is parameterized by a security parameter $\secp$; especially, a transaction is declared stable if and only if it is in a block that is more than $\secp$ blocks deep in the ledger.
  \item \textbf{Liveness}. (New transactions included eventually). If all honest nodes in the system attempt to include a certain transaction then, after the passing of time corresponding to $\mu$ slots (called the transaction confirmation time), all nodes, if queried and responding honestly, will report the transaction as stable.
\end{itemize}

\subsubsection{Properties}

Imprecisely speaking, as discussed in \cite{C:KRDO17}, we show that \textit{persistence} and \textit{liveness} can be derived from the following three elementary properties provided that protocol $\Pi$ derives the ledger from a data structure in the form of a blockchain.
In this work, we focus on the quantum-resistant PoS blockchain consensus and ignore the quantum-resistant transactions. Hence, we focus on the three elementary properties, \ie, common prefix, chain growth, and chain quality. The properties of persistence and liveness can be derived from the following three elementary properties.

\begin{itemize}
  \item \textbf{Common Prefix (CP or chain consistency)}; with parameters $\compp\in \N$. The chains $\chainC_1$ and $\chainC_2$ possessed by two honest parties at the onset of the slots $\slot_1< \slot_2$ are such that $\chainprefix_1 \preceq \chainC_2$, where $\chainprefix_1$ denotes the chain obtained by removing the last $\compp$ blocks from $\chainC_1$, and $\preceq$ denoted the prefix relation.

  \item \textbf{Chain Growth (CG)}; with parameters $\cgp\in (0, 1]$, $s \in \N$. Consider the chains $\chainC_1$, $\chainC_2$ processed by two honest parties at the onset of two slots $\slot_1$, $\slot_2$ with $\slot_2$ at least $s$ slots ahead of $\slot_1$. Then it holds that $\strlen(\chainC_2)-\strlen(\chainC_1)\geq \cgp\cdot s$. We call $\cgp$ the speed coefficient.

  \item \textbf{Chain Quality (CQ)}; with parameters $\cqp\in (0,1]$ and $\ell\in N$. Consider any portion of length at least $\ell$ of the chain possessed by an honest party at the onset of a round; the ration of blocks originating from the adversary is at most $1-\cqp$. We call $\cqp$ the chain quality coefficient.
\end{itemize}

These security properties have been adopted in many subsequent blockchain designs, such as \cite{EC:PasSeeshe17,C:BMTZ17,PODC:PasShi17,AC:PasShi17,EC:BGMTZ18,CCS:BGKRZ18}.
}

\subsection{Transaction Ledger Properties}

A protocol $\Pi$ implements a robust transaction ledger provided that the ledger that $\Pi$ maintains is divided into ``blocks'' (assigned to time slots) that determine the order with which transactions are incorporated in the ledger. It should also satisfy the following two properties.

\begin{itemize}
  \item \textbf{Persistence}. (Past (or stable) transactions in the ledger are immutable). Once a node of the system proclaims a certain transaction $\tx$ as \textit{stable}, the remaining nodes, if queried, will either report $\tx$ in the same position in the ledger or will not report as stable any transaction in conflict to $\tx$. Here the notion of stability is a predicate that is parameterized by a security parameter $\secp$; especially, a transaction is declared stable if and only if it is in a block that is more than $\secp$ blocks deep in the ledger.
  \item \textbf{Liveness}. (New transactions included eventually). If all honest nodes in the system attempt to include a certain transaction then, after the passing of time corresponding to $\mu$ slots (called the transaction confirmation time), all nodes, if queried and responding honestly, will report the transaction as stable.
\end{itemize}

\begin{definition}[Fork]
We define the notion of a \textit{fork} with respect to blockchains. Let $\blockB$ be some blockchain. A fork \wrt $\blockB$ is a sequence of valid blocks that extends some prefix of blockchian $\blockB$ instead of extending $\blockB$ directly from its end.
\end{definition}

In other words, a fork is a sequence of valid blocks that starts extending the chain at some block which is not the most recently added block in $\blockB$.

\draft{
\subsection{PoS Protocol}

%\subsection{Our Blockchain Protocol}
In the next two subsections, to describe the post-quantum PoS protocol, we follow the framework of blockchain based PoS presented by~Scafuro, Siniscalchi, and Visconti~\cite{PKC:ScaSinVis19} which followed the verbatim from~\cite{EC:PasSeeshe17,TCC:GoyGoy17}. In more detail, a blockchain protocol consists of 4 polynomial-time algorithms
$$
(\UpdateState, \GetRecords, \Broadcast, \GetHash).
$$
\begin{itemize}
  \item $\bar{\state}\gets\UpdateState(1^\secp, \state)$: it takes as input the security parameter $\secp$, state $\state$ and outputs the update state $\bar{\state}$. More concretely,  before executing the cryptographic PoS puzzle, each stakeholder $U_i$ in the setting first to initialize his own state $\state_i:=h_{i-1}=\hashH(\blockB_{i-1})$.

  \item $\blockB\gets \GetRecords(1^\secp, \bar{\state})$: it takes as input the security parameter $\secp$ and state $\bar{\state}$. It outputs the longest ordered sequence of valid blocks $\blockB$ (or simply blockchain) contained in the state variable, where each block in the chain itself contains an unordered sequence of records messages. More concretely, depending on our settingss, if the stakeholder $U_i$ holds at least 2\% of total stakes, then he will automatically become the elector $E_i$. Then, the elector $E_i$ proceeds the algorithm as follows:

      \begin{enumerate}
        \item the elector $E_i$ is enable to become the leader who has the right to create the next block with the quota stake $\stake_i$ and the probability $\probld_i = {\stake_i}/{\sum_{k=1}^n \stake_k}$ for $i\in [N]$.

        \item next, each elector $E_i$ begins to execute his quantum-resistant signature scheme       $\sigma_i=\uSign_{\sk_i}(\state_i:=\hashH(\blockB_{i-1}),\data_i,\slot_i)$ under $\sk_i$ corresponding to the elector $E_i$ generating the block.

        \item then, each elector is struggling to become the next block creator by testing whether satisfies the following inequality, \ie, cryptographic PoS puzzle
\begin{equation}\label{eq:pos}
  \hashH(\state_i:=\hashH(\blockB_{i-1}), \data_i, \slot_i, \pk_i, \sigma_i)< \stake_i \cdot\tgtT.
\end{equation}
where the target value $\tgtT$ is fixed and ``posted on the sky'', but different elector $E_i$ has different $\stake_i$, thus, if the elector who has more stakes, then $\stake_i \cdot\tgtT$ is larger and he is more likely to be the creator for the next block.

     \item  if the elector $E_i$ passes the inequality~\ref{eq:pos} firstly, then he becomes the leader $\leader_i $ and is entitled to the new coming block $\blockB$.

      \end{enumerate}

  \item $\Broadcast(1^\secp, \record)$: it takes as input a security parameter $\secp$ and a message $\msg$, and broadcasts the message over the network to all nodes executing the blockchain protocol. It does not give any output.

  \item $\GetHash(1^\secp, \blockB)$: it takes as input a security parameter $1^{\secp}$ and a blockchain $\blockB$, and outputs the description of a collision-resistant hash function $\hfuncH(\cdot)$ publicly available in $\blockB$.
\end{itemize}

}

\subsection{Analysis of Chain Growth}\label{Appsubsec:chaingrowth}

\draft{
Intuitively, the chain growth property states that the chains of honest players should grow linearly to the number of rounds. In our setting, we are mimicking the bitcoin backbone by using a unique signature to act the role of a cryptographic puzzle solution. Hence, in the following proof, we can follow the proof of the strategy of \cite{EC:GarKiaLeo15} to analyze the property of chain growth.

\begin{definition}[Chain Growth Property ($\Qcg$), adopted from~\cite{EC:GarKiaLeo15}]
The chain growth property $\Qcg$ with parameter $\hstkratio:=1-\astkratio\in \R$ and round $\rounds\in \N$ states that for any honest party $P$ with chain $\chainC$, it holds that for any $\rounds$ there are at least $\hstkratio\cdot \stake$ blocks added to the chain of $P$.
\end{definition}

\begin{lemma}[Chain Growth Lemma]
If an honest party has a chain of length $\chainlength$ at round $\roundr$, then every honest party has adopted a chain of length at least $\chainlength+\sum^{\rounds-1}_{i=\roundr}X_i$ by round $\rounds\geq \roundr$.
\end{lemma}
}

\par\noindent\textbf{Proof of Lemma~\ref{lemma:chain-growth}}.
Below, we prove Lemma~\ref{lemma:chain-growth} following the methodology of Bitcoin backbone~\cite{EC:GarKiaLeo15}.
\begin{proof}
By induction on $\rounds-\roundr\geq 0$. For the basis $(\rounds=\roundr)$, observe that if at round r an honest party has a chain $\chainC$ of length $\chainlength$, then that party broadcast $\chainC$ at a round earlier than $\roundr$. It follows that
every honest party will receive $\chainC$ by round $\roundr$.

For the inductive step, note that by the inductive hypothesis every honest party has received a chain of length at least $\chainlength'=\chainlength+\sum_{i=\roundr}^{\rounds-2}X_i$ by round $\rounds-1$. When $X_{\rounds-1} = 0$ the statement follows directly, so assume $X_{\rounds-1}= 1$. Observe that every honest party queried the oracle with a chain of length at least $\chainlength'$ at round $\rounds-1$. If follows that all honest parties successful at round $\rounds-1$ broadcast a chain of length at least $\chainlength'+1$. Since $\chainlength'+1=\sum_{i=\roundr}^{\rounds-1}X_i$, this completes the proof.
\end{proof}

%\begin{theorem}[Chain Growth]\label{theorem:chain-growth}%\zlinote{refer to Ourobours}
%The protocol satisfies the chain growth property with parameters $\hstkratio:=1-\astkratio$, $\rounds\in \N$ throughout an epoch of $R$ slots with probability at least $1-\exp(-\Omega(\sysp^2\rounds)+\ln R)$ aghast an adversary holding an $\astkratio-\sysp$ portion of the total stake for system parameter $\sysp\in \set{0,1}$.
%\end{theorem}

\par\noindent\textbf{Proof of Theorem~\ref{theorem:chain-growth}}.
Below we detail the proof of Theorem~\ref{theorem:chain-growth}. But before proving the above Theorem~\ref{theorem:chain-growth}, we first define the \textit{hamming weight} $\HW_a(\astkratio)$ to be the event that the Hamming weight ratio of the characteristic string that corresponds to the slots $[a, a+s-1]$ is no more than $\astkratio$. Below, we provide the detailed analysis.
\begin{proof}
We assume that the \textit{adversarial stake} is $\astkratio-\sysp$, each of the $k$ slots has probability $\astkratio-\sysp$ being assigned to the adversary and thus the probability that the Hamming weight is more than $\astkratio\cdot \rounds$ drops exponentially in $\rounds$. In particular, armed with the Chernoff bound in Theorem~\ref{theorem:CHbound}, we have the following result:
\begin{equation*}
  \Pr[\HW_a(\astkratio)]\geq 1-\exp(-2\sysp^2\cdot \rounds).
\end{equation*}
Given the above, we know that when $\HW_a(\astkratio)$ happens there will be at least $(1-\astkratio)\cdot \rounds$ honest slots in the period of $\rounds$ rounds. Given that each honest slot enables an honest party to produce a block, all honest parties will advance by at least that many blocks. Using a union bound, it follows
that the speed coefficient can be set to $\hstkratio=1-\astkratio$ and it is satisfied with probability at least $1-\exp(-\Omega(\sysp^2\rounds)+\ln R)$.
\end{proof}

\subsection{Analysis of Chain Quality}\label{Appsubsec:chainquality}

\draft{
The property of chain quality aims at expressing
the number of honest blocks' contributions that are contained in a sufficiently long and continuous part of an honest chain. In our work, we follow the same spirit of Ouroboros to define the security properties for our proposed a quantum resistant PoS blockchain protocol.

\begin{definition}[Chain Quality Property $\Qcq$]
The chain quality $\Qcq$ with parameters $\mu\in \R$ and $\chainlength\in \N$ state that for any honest party $P$ with chain $\chainC$, it holds that for any $\chainlength$ consecutive blocks of $\chainC$ the ratio of honest blocks is at least $\mu$.
\end{definition}

%\begin{lemma}[Chain Quality Lemma]
%\zlinote{Do not need this lemma}
%\end{lemma}

\begin{theorem}[Chain Quality]
Let $\astkratio-\sysp$ be the adversarial stake ratio. The protocol satisfies the chain quality property with parameters $\mu\cdot (\astkratio-\sysp)=\astkratio/(1-\astkratio)$ and $\chainlength\in \N$ through an epoch of $R$ slots with probability at least
\begin{equation*}
  1-\exp(-\Omega(\sysp^2\cdot (\astkratio\cdot\chainlength))+\ln R).
\end{equation*}

\end{theorem}
}

\par\noindent\textbf{Proof of Theorem~\ref{theorem:chain-quality}}.
 Below we sketch the proof of Theorem~\ref{theorem:chain-quality}.

\begin{proof}[Sketched Proof]
Firstly, from the proof for chain growth in Theorem~\ref{theorem:chain-growth}, we know that with high probability a segment of $\chainlength$ rounds will involve at least $(1-\astkratio)\cdot\chainlength$ slots with honest leaders; hence the resulting chain must advance by at least $(1-\astkratio)\cdot\chainlength$ blocks.

Furthermore, by similar reasoning, the adversarial parties are associated with no more than $\astkratio\cdot \chainlength$ slots, and thus can contribute no more than $\astkratio\cdot \chainlength$ blocks to any particular chain over this period. It follows that the associated chain possessed by any honest party contains a
fraction $\astkratio/(1-\astkratio)$ of adversarial blocks with probability $1-\exp(-\Omega(\sysp^2\cdot (\astkratio\cdot\chainlength))+\ln R)$.
\end{proof}

\subsection{Analysis of Common Prefix}\label{Appsubsec:commonprefix}
Below, we detail how to proof the property of the common prefix. In PoS, blockchain fork is an inevitable problem. In this case, we can not continue to prove this property following the spirit of \cite{EC:GarKiaLeo15}. On the contrary, we adopt the proof strategy of Ouroboros~\cite{C:KRDO17} to analyze the property of common prefix.
Furthermore, based on the property called ``common prefix'' in~\cite{EC:GarKiaLeo15}, it is shown that with overwhelming probability in the security parameter, the parties terminate with the same output, while using the ``chain quality'' property, it is shown that if all the honest parties start with the same input, the corrupt parties cannot overturn the majority bit, which corresponds to the honest parties' input. The number of tolerated misbehaving parties in this protocol is strictly below $n/3$, a sub-optimal resiliency due to the low chain quality of the underlying blockhain protocol. The maximum resiliency that can be expected is $n/2$, something that can be shown by easily adapting the standard argument for the necessity of honest majority.
\begin{definition}[Fork $\forkF\to \strw$]
Let $\forkF\vdash \strw$ be a fork for a string $\strw\in\set{0,1}^n$. We say that $\forkF$ is covert if the labeling $\ell: V\to \set{0,1, \cdots,}$ is injective. In particular, no adversarial index is labeled by more than one node.
\end{definition}

\begin{definition}
We say that a string $\strw$ is covertly forkable if there is a flat covert fork $\forkF\to \strw$.

\end{definition}

\begin{definition}[Divergence]
Let $t$ be a tine of $\forkF$, and let $\forkF$ be a fork for string $\strw\in \set{0,1}^*$. For two viable tines $t_1$ and $t_2$ of $\forkF$, define their divergence to be the quantity
\begin{equation*}
  \strdiv(t_1, t_2)=\min_t(\strlen(t_i)-\strlen(t_1 \cap  t_2 )),
\end{equation*}
where $t_1 \cap  t_2$ denotes the common prefix of $t_1$ and $t_2$.
We overload this notation by defining divergence for $\forkF$ as the maximum over all pairs of viable tines:
\begin{equation*}
  \strdiv(\forkF)=\max_{t_1,~ t_2~ viable~tines~ of ~\forkF} \strdiv(t_1, t_2).
\end{equation*}
Finally, define the divergence of $w$ to be the maximum such divergence over all possible forks for $\strw$:
\begin{equation*}
  \strdiv(\strw)=\max_{\forkF \vdash \strw} \strdiv(\forkF).
\end{equation*}
Observe that if $\strdiv(t_1, t_2)\leq \compp$ and $\strlen(t_1)\leq \strlen(t_2)$, the tine  $t_1^{\lceil \compp}$  is  a prefix of $t_2$.

\end{definition}

\begin{theorem}
Let $\strw\in\set{0,1}^*$. Then there is forkable substring $\breve{\strw}$ of $\strw$ with $\abs{\breve{\strw}}\geq \strdiv(\strw)$.

\end{theorem}
Regarding the rigorous security proof, please refer to \cite[Theorem~4.26]{C:KRDO17} for more details.

\draft{
\begin{definition}[Common Prefix Property ($\Qcp$)]
The common prefix property $\Qcp$ with parameter $\secp\in \N$ states that for any pair of honest players $P_1$, $P_2$ adopting the chains $\chainC_1$, $\chainC_2$ at round $\roundr_1\leq \roundr_2$ respectively, it holds that $\chainprefix_1 \preceq \chainC_2$ and $\chainprefix_2 \preceq \chainC_1$.
\end{definition}

\begin{lemma}[Common Prefix Lemma]
If assume a typical execution and consider two chains $\chainC_1$ and $\chainC_2$. If
$\chainC_1$ is adopted by an honest party ar round $\roundr_1$, and $\chainC_2$ is either adopted by an honest party at round $\roundr$ or diffused at round $\roundr$ and has $\strlen(\chainC_2)\leq \strlen(\chainC_1)$, then $\chainprefix_1 \preceq \chainC_2$ and $\chainprefix_2 \preceq \chainC_1$ for $\compp$ consecutive blocks and $\secp$ consecutive rounds, \ie, $\secp\leq \compp/2 p$.
\end{lemma}
Below we sketch the proof and please refer to ~\cite[Lemma~14]{EC:GarKiaLeo15} for more concrete proof.
Assume, towards a contradiction, an execution in which the assumptions of the lemma hold, but either $\chainprefix_1 \npreceq \chainC_2$ or $\chainprefix_2 \npreceq \chainC_1$ for $\compp\geq 2\secp p$.
Consider the last block on the common prefix of $\chainC_1$ and $\chainC_2$ that was computed by an honest party and $\roundr^*$ be the round on which it was computed (if no such block exists for let $\roundr^*=0$). Define the set of rounds $\setS=\set{i: \roundr^*< i< \roundr}$. We claim that
\begin{equation*}
  Z(S)\geq Y(S).
\end{equation*}
However, $Z(S)\geq Y(S)$ contradicts  $Z(S) < Y(S)$.

\begin{theorem}[Common Prefix]
The probability of the protocol, when expected with a $(1-\sysp)/2$ fraction of adversarial stake, conflicts the common prefix property with parameter $\compp$ throughout an epoch of $R$ slots is no more that $\exp(-\Omega(\sqrt{\compp})+\ln{R})$; the constant hidden by the $\Omega(\cdot)$ notation depends only on $\sysp$.
\end{theorem}
}

\par\noindent\textbf{Proof of Theorem~\ref{theorem:common-prefix}}.
Below we detail the proof of Theorem~\ref{theorem:common-prefix}.
\begin{proof}
Observe that an execution of our proposed protocol conflicts the common prefix property with parameters $\compp$, $R$ precisely when the fork $\forkF$ induced by this execution has $\strdiv(\forkF)\geq \compp$.

Thus we wish to show that the probability that $\strdiv(\strw)\geq \compp$, there is a forkable substring $\breve{\strw}$ of length at least $\compp$. Thus, for $\strw\in\set{0,1}^n$
\begin{eqnarray*}
 &~&\Pr[\text{common~prefix~violation}]\\
  &=& \Pr\left[
                                        \begin{array}{c}
                                          \exists~\astkratio, \beta \mbox{~so~that~}\\
                                          \astkratio+\compp-1\leq \beta \mbox{~and}\\
                                          \strw_{\astkratio},\cdots,\strw_{\beta} \mbox{is~forkable} \\
                                        \end{array}
                                      \right]
   \\
   &=& \sum_{1\leq \astkratio\leq R } \sum_{\astkratio+\compp-1\leq \beta\leq R}
   \Pr[\strw_{\astkratio},\cdots,\strw_{\beta} \mbox{~is~forkable}]
\end{eqnarray*}

Recall that the characteristic string $\strw\in\set{0,1 }^R$ for such an execution of protocol is determined by assigning each $\strw_i=1$ independently with probability $(1-\sysp)/2$. Note that, $\Pr[\strw~is~forkable]=2^{-\Omega(\sqrt{n})}$ for $\strw\in \set{0,1}^n$ and $\strw_i=1$ with probability $(1-\sysp)/2$ for $\sysp\in (0,1)$. In this case, the probability that a string of length $t$ drawn from this distribution is forkable is no more than $\exp(-c\sqrt{t})$ for a positive constant $c$. Note that for any $\astkratio\geq 1$,
\begin{eqnarray*}
% \nonumber to remove numbering (before each equation)
  \sum^R_{t=\astkratio+\compp-1} e^{-c\sqrt{t}} &\leq& \int_{\compp-1}^{\infty} e^{-c\sqrt{t}}dt \\
   &=& (2/c^2)(1+c\sqrt{\compp-1})e^{-c\sqrt{\compp-1}}\\
   &=&  c^{-\Omega(\sqrt{\compp})}
\end{eqnarray*}

and it follows that the $\sum$ above is $\exp(-\Omega(\sqrt{t}))$. Thus
\begin{eqnarray*}
% \nonumber to remove numbering (before each equation)
  \Pr[\text{common~prefix~violation}] &\leq& R\cdot \exp(-\Omega\sqrt{\compp}) \\
  &\leq & \exp(\ln R-\Omega(\sqrt{\compp}))
\end{eqnarray*}
as desired.
\end{proof}
